# Supplementary material for: Swift UVOT observations of the 2015 outburst of V404 Cygni
Source: arXiv:1809.03237 ancillary file (2019-08-12)
Supplement: Supplementary file 1 [file V404_supp.pdf]

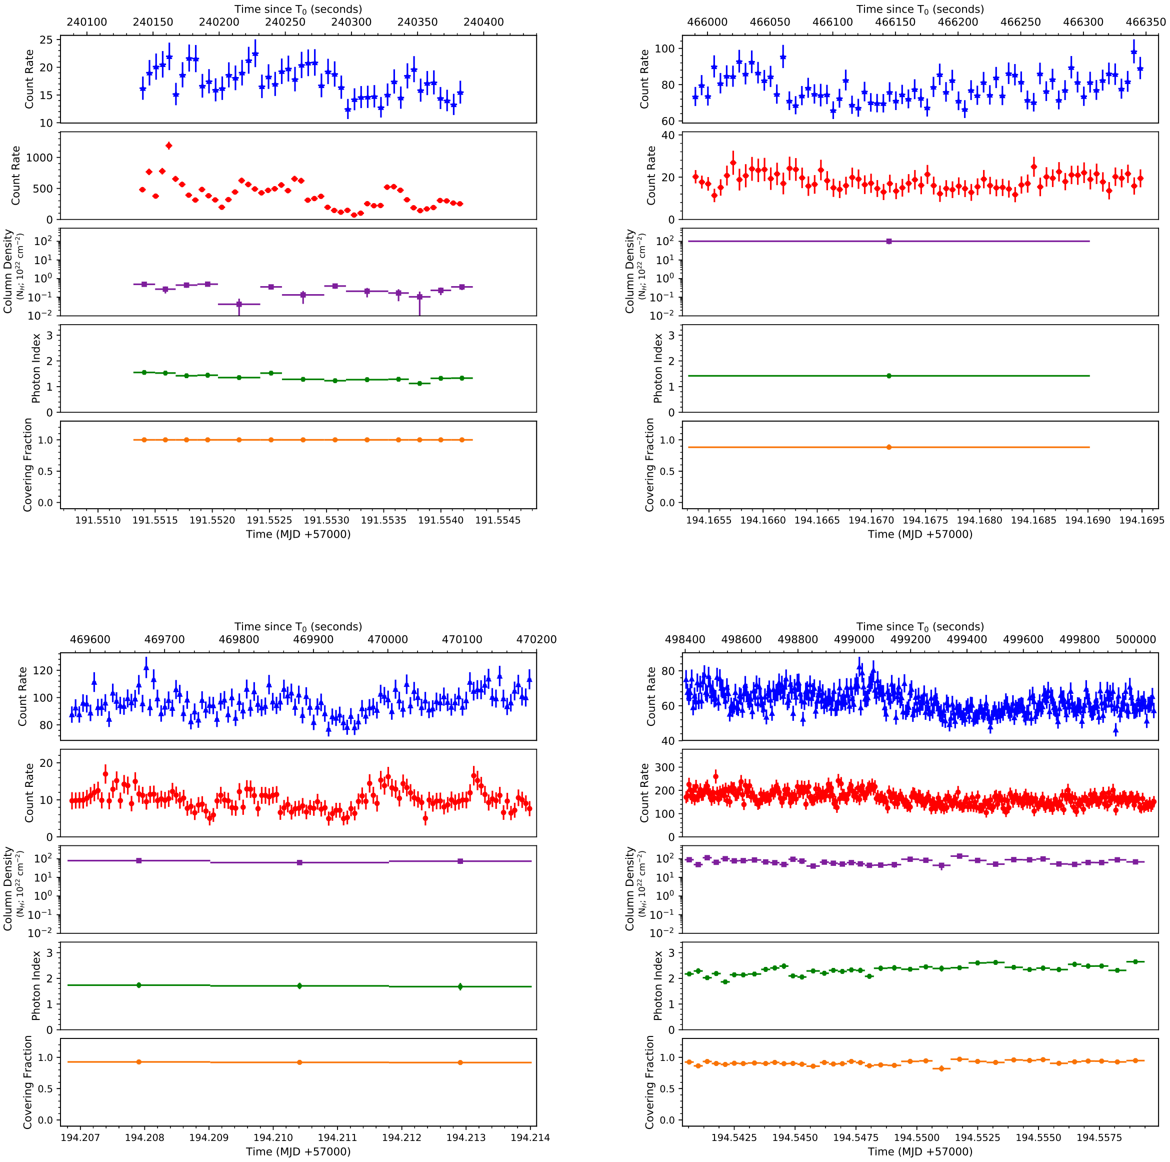


**Figure S.1.** High time resolution observations of V404 Cygni taken in the *u*-band (blue triangles; top panel) and 0.5 − 10 keV X-ray (red circles; second panel). For each segment, the X-ray data has been resampled to have the same bin times as the *u*-band observations. In the final three panels we show the results of the time resolved X-ray spectral fitting performed by Motta et al., (2017) displaying the resulting neutral hydrogen column density ($N_H$; third panel), the power-law photon index ($\Gamma$; fourth panel) and the partial covering fraction (final panel). For the X-ray spectral analysis, we only provide the results where the parameter could be constrained and is not an upper limit. For the partial covering fraction, a value of 1 indicates that the absorber is uniform. The error bars for many points are smaller than the markers.

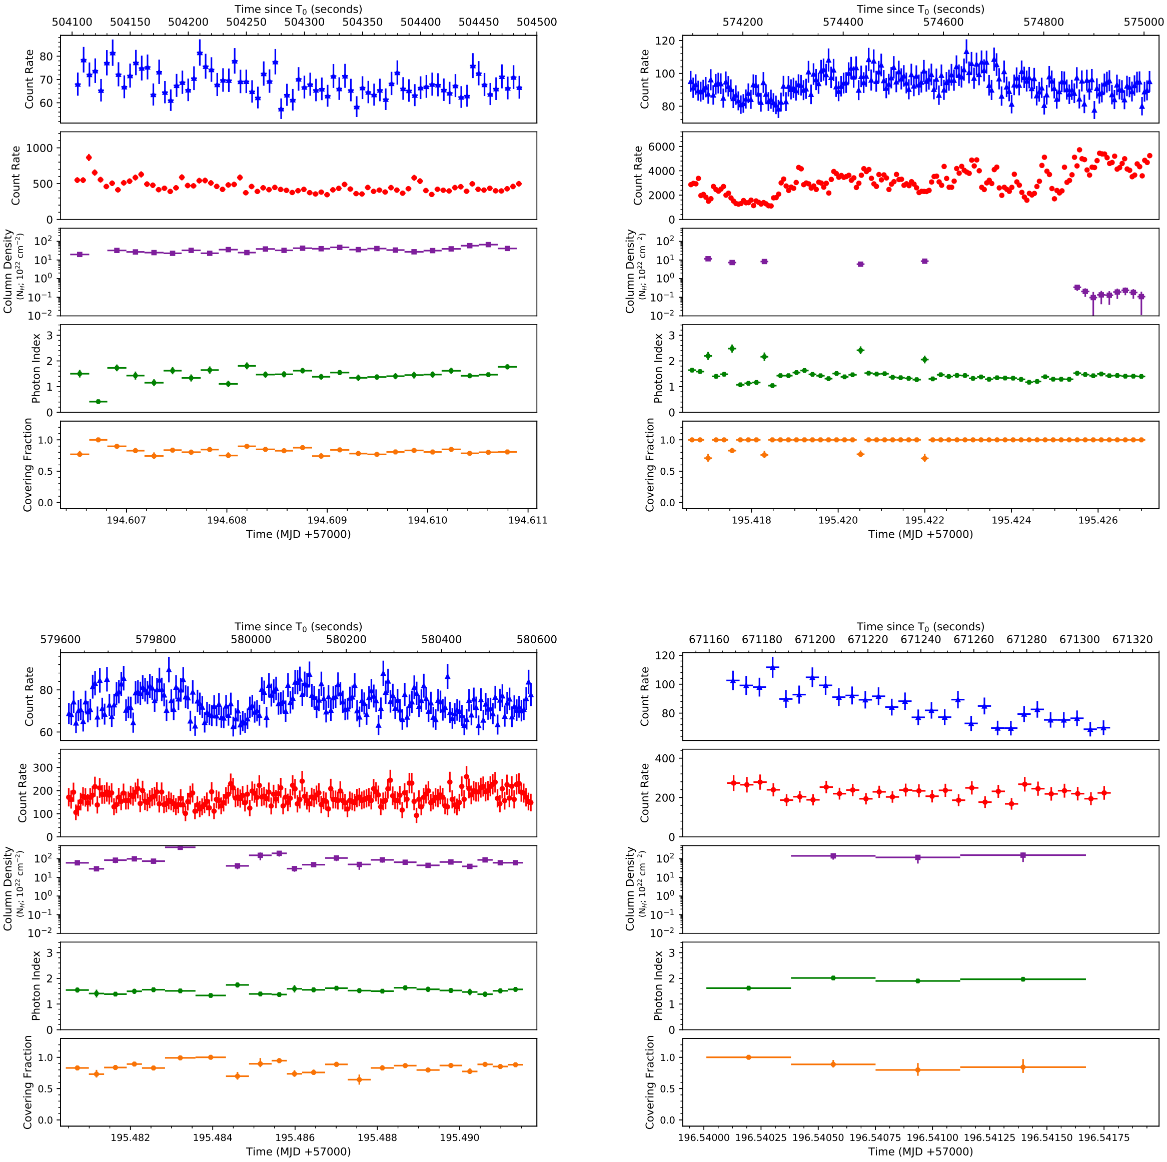


**Figure S.1 (Cont.).**

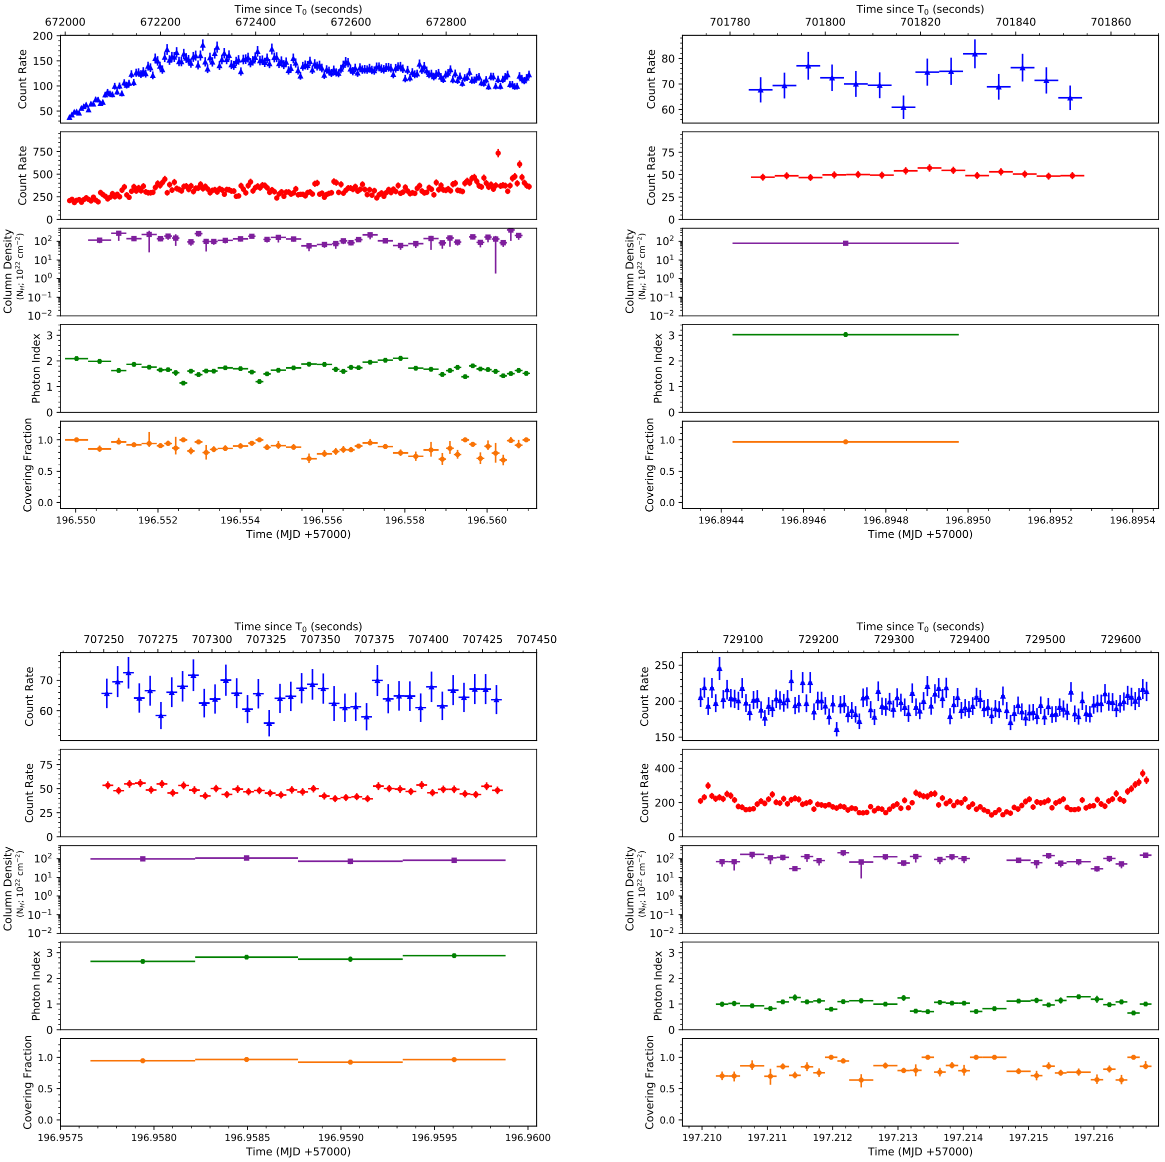


**Figure S.1 (Cont.).**

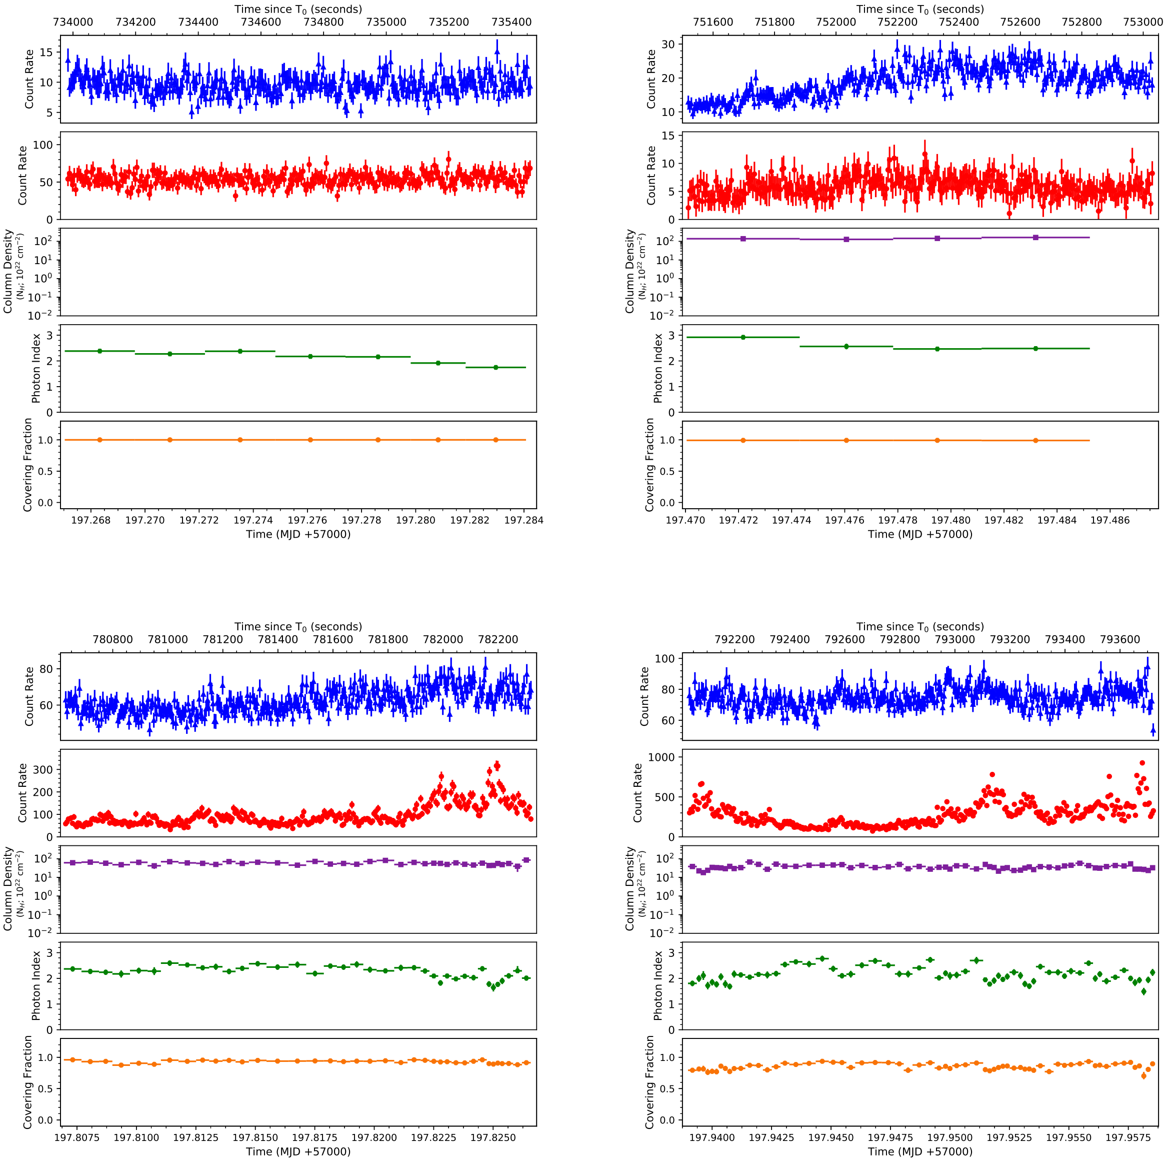


**Figure S.1 (Cont.).**

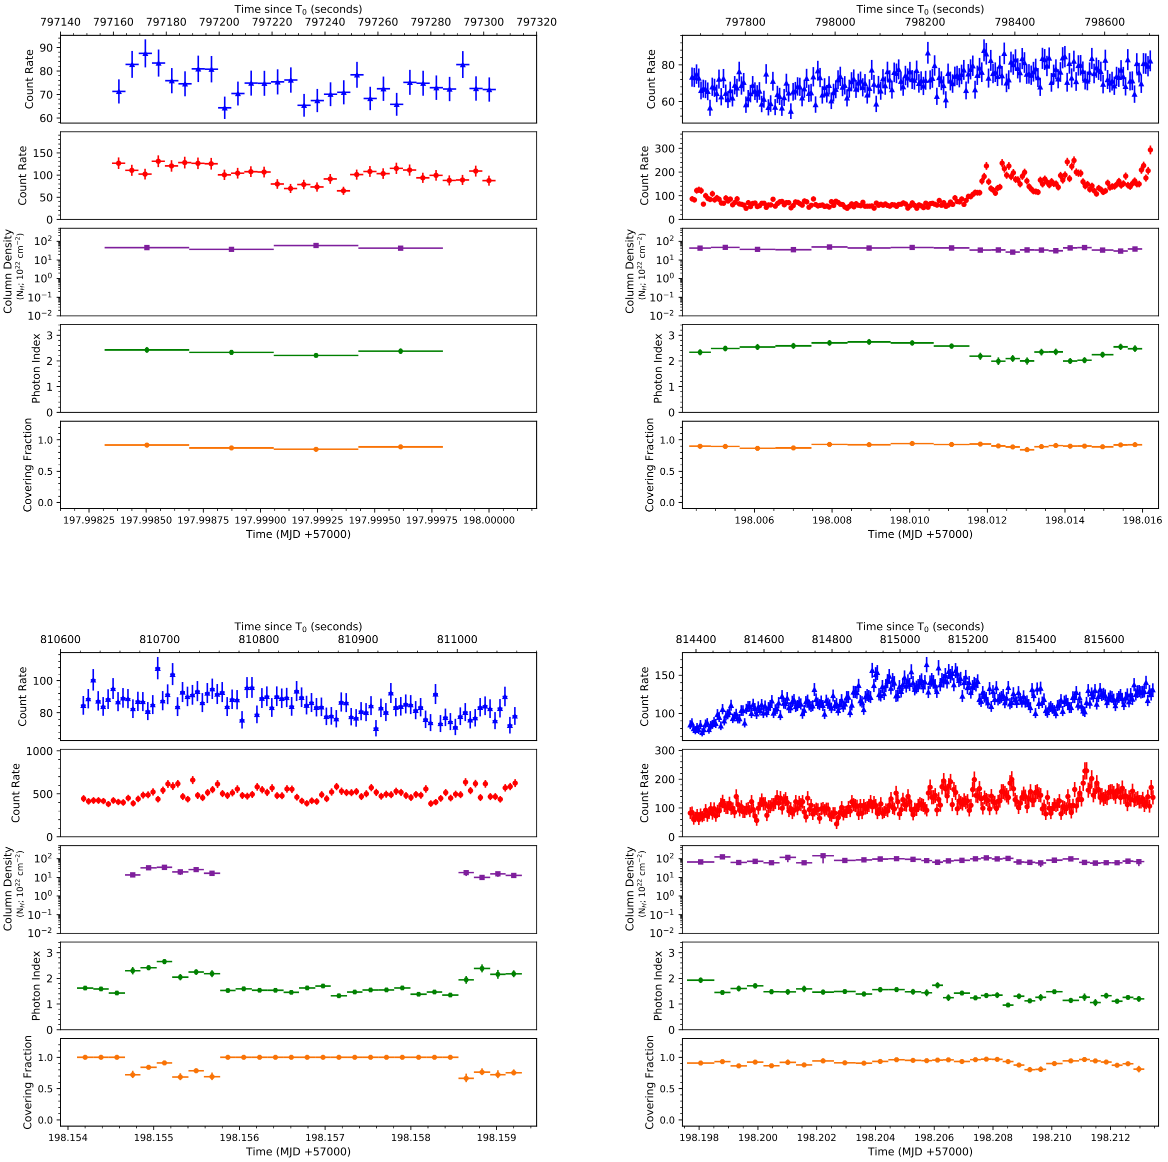


**Figure S.1 (Cont.).**

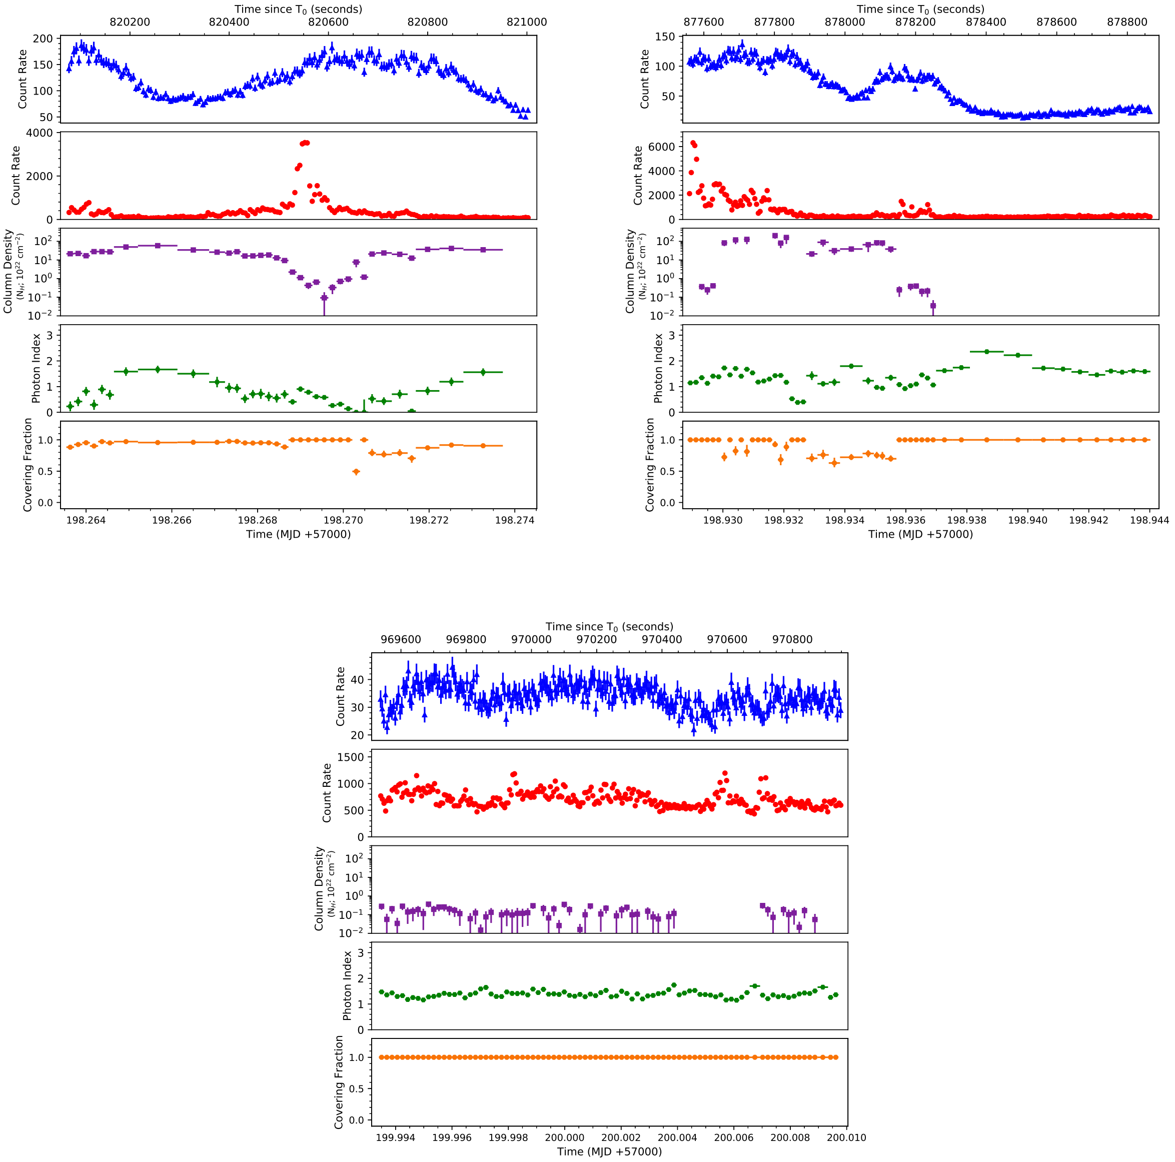


**Figure S.1 (Cont.).**

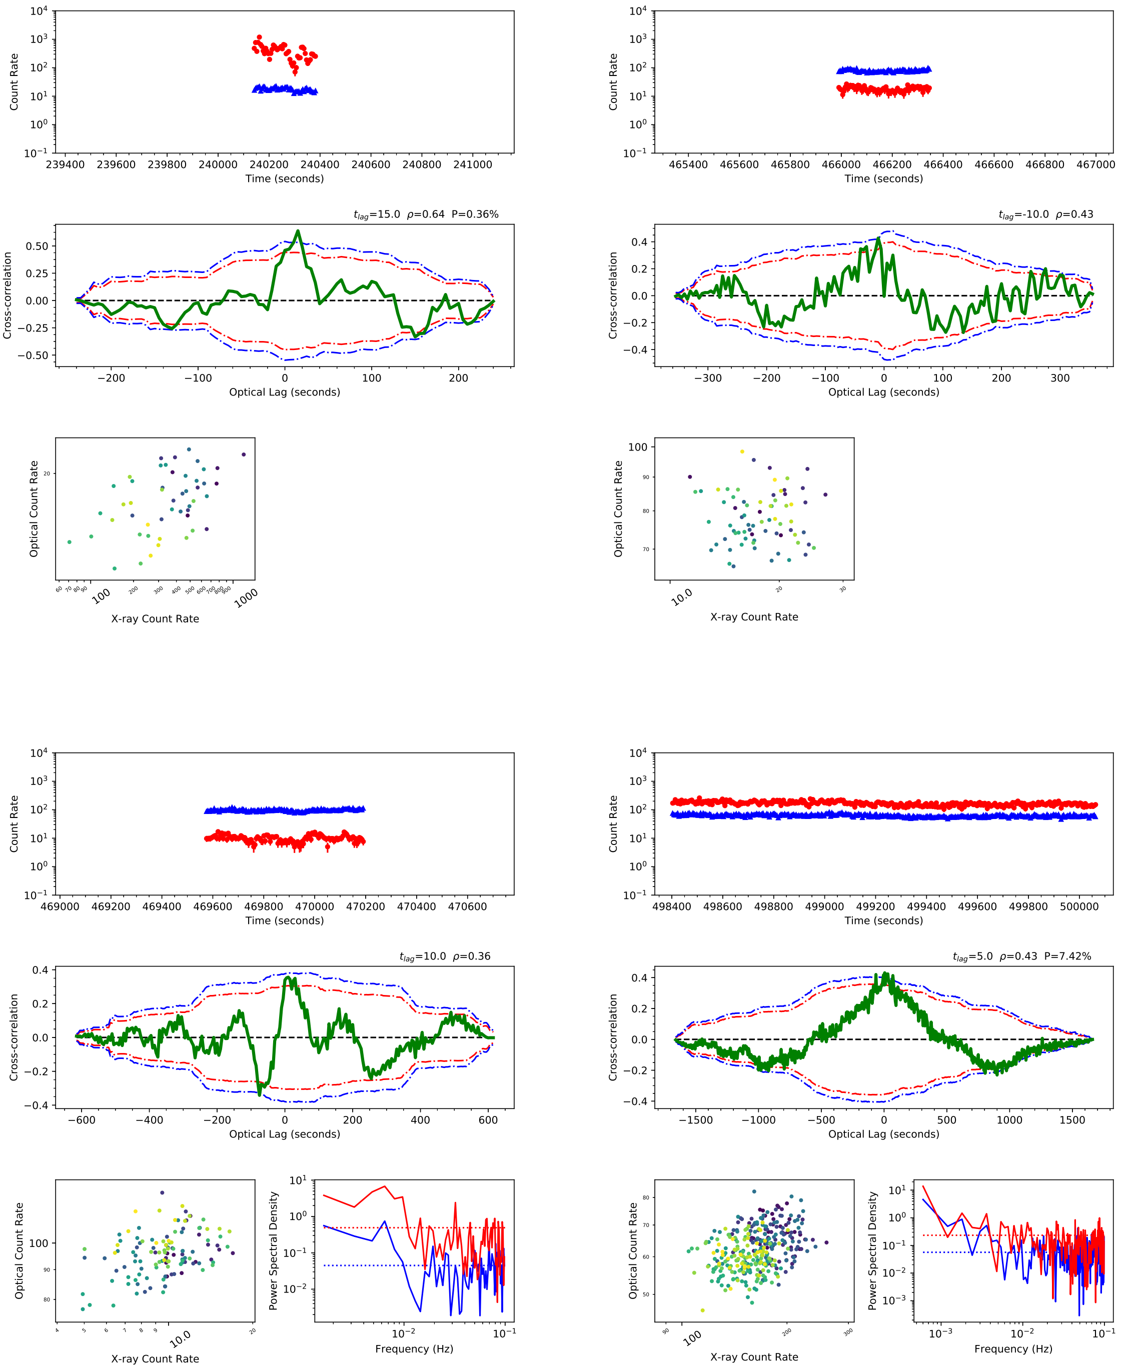


**Figure S.2.** Time sliced observations of the optical and X-ray observations of V404 Cygni. For each time segment there are three panels. The top panel displays the 5s binned $0.5-10$ keV X-ray (red circles) and $u$-band (blue triangles) light curves. The middle panel displays the optical lag (green solid line) determined by cross correlating the $u$-band and X-ray light curve for that particular segment. The blue, and red dotted-dashed lines delineate the 0.5, 2.5, 97.5 or 99.5 per cent values of the cross correlation distribution determined through a Monte Carlo simulation. In the top right above the middle panel, we give the optical lag time and coeffcient at the peak of the cross correlation function and the probability of it occurring by chance considering the multiple cross correlations performed for that segment (provided when the value is $< 10$ per cent). The lower left panel displays the optical count rate ($u$-band) versus the X-ray $(0.5-10\,\mathrm{keV})$ count rate, where the colour represents the time of observations (dark purple being the earliest time, through green with the latest times displayed in yellow. For some epochs the lower panel contains a lower right panel, which displays the power density spectrum of the $u$-band (blue) and X-ray (red) light curve. This panel is only given when the top panel contains $\geqslant 100$ data points (equivalent to a duration of 500 s). The dotted lines in their corresponding colours indicate the expected constant Poissonian white noise contribution for the two bands. All top panels have the same time width and count rate range in order for ease of comparison of duration and brightness between different panels.

© 0000 RAS, MNRAS **000**, 000–000

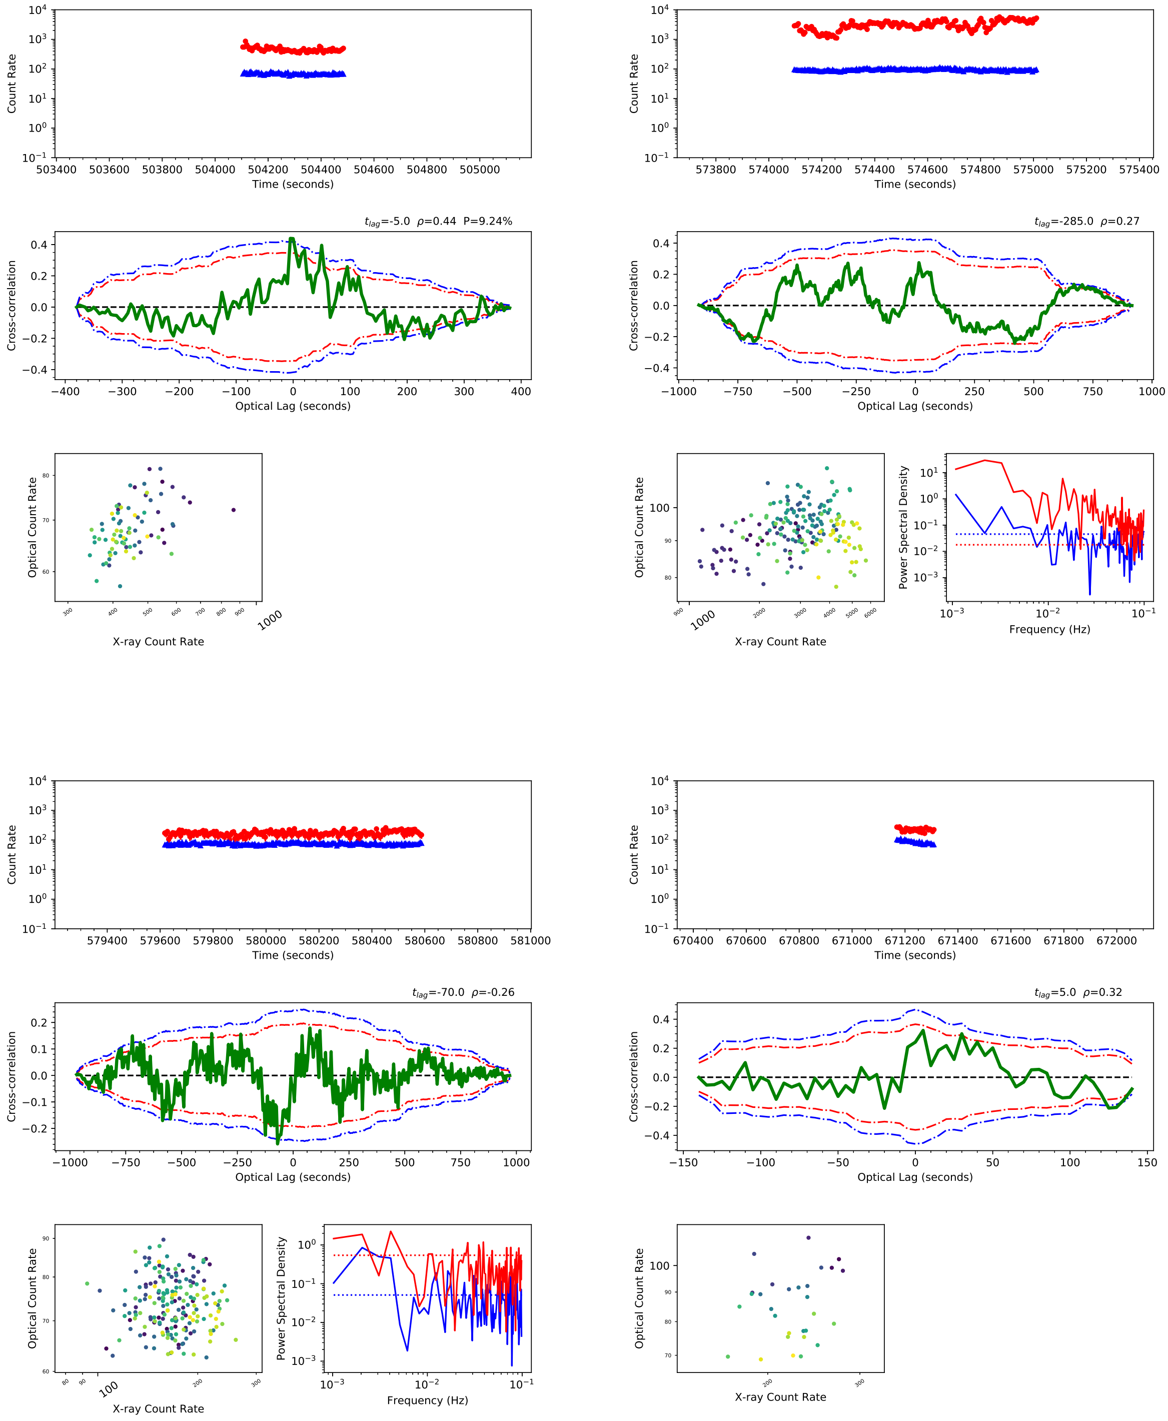


**Figure S.2 (Cont.).**

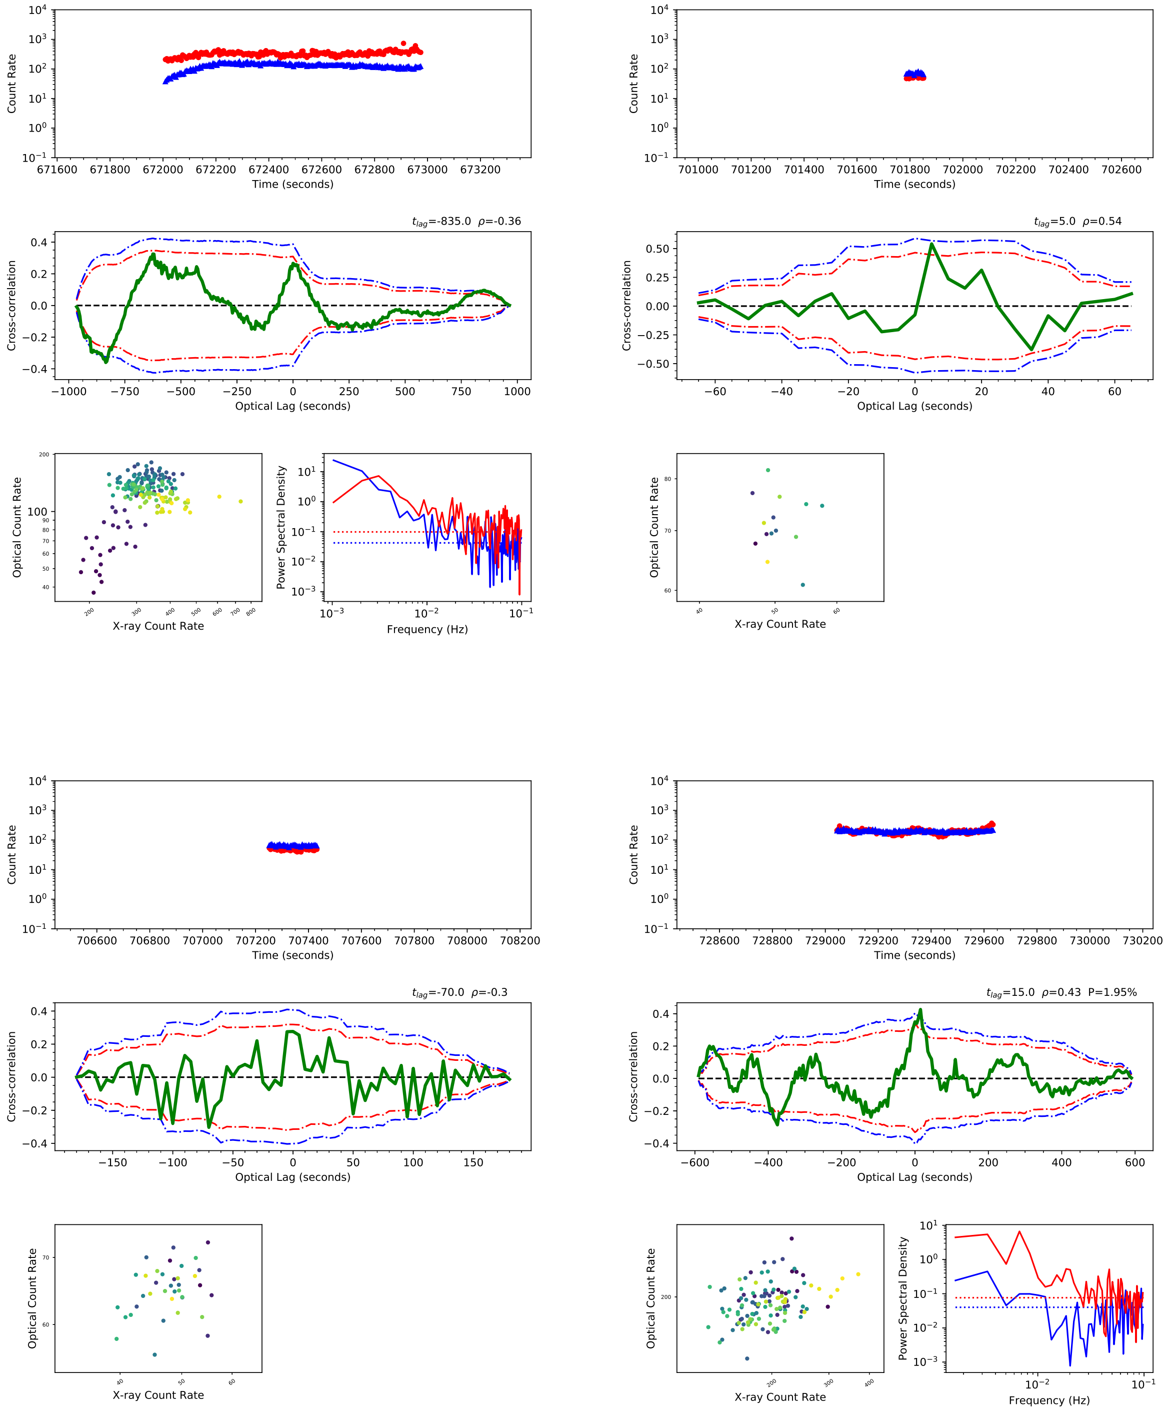


**Figure S.2 (Cont.).**

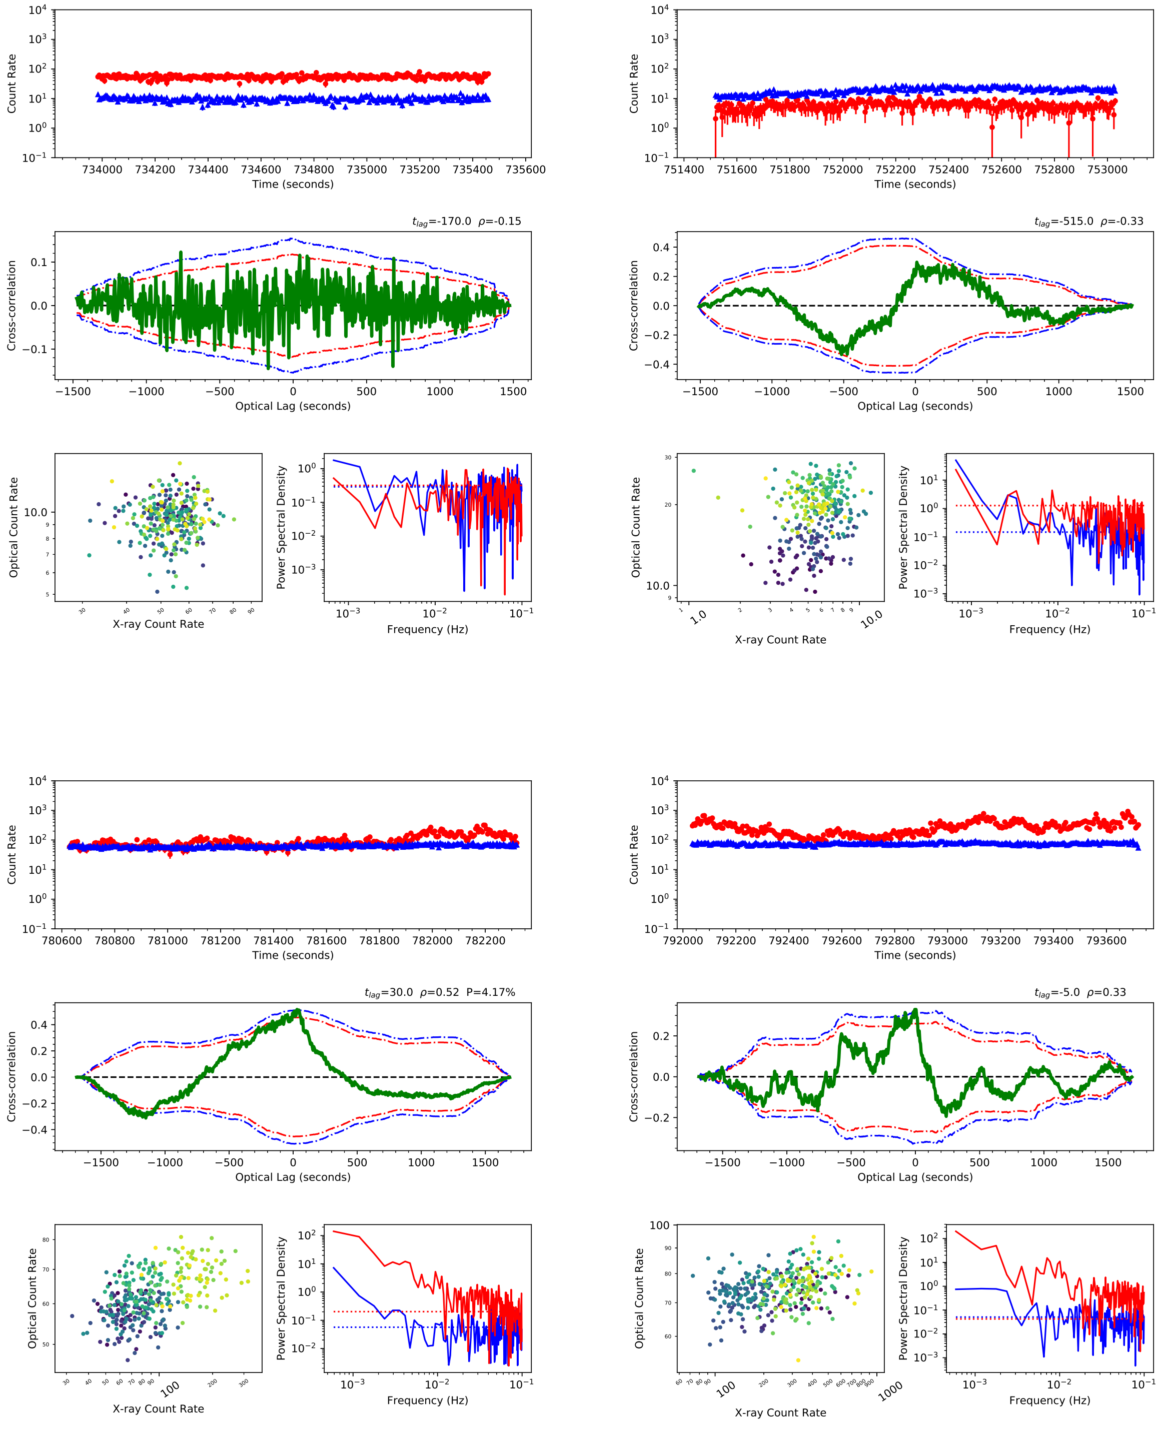


**Figure S.2 (Cont.).**

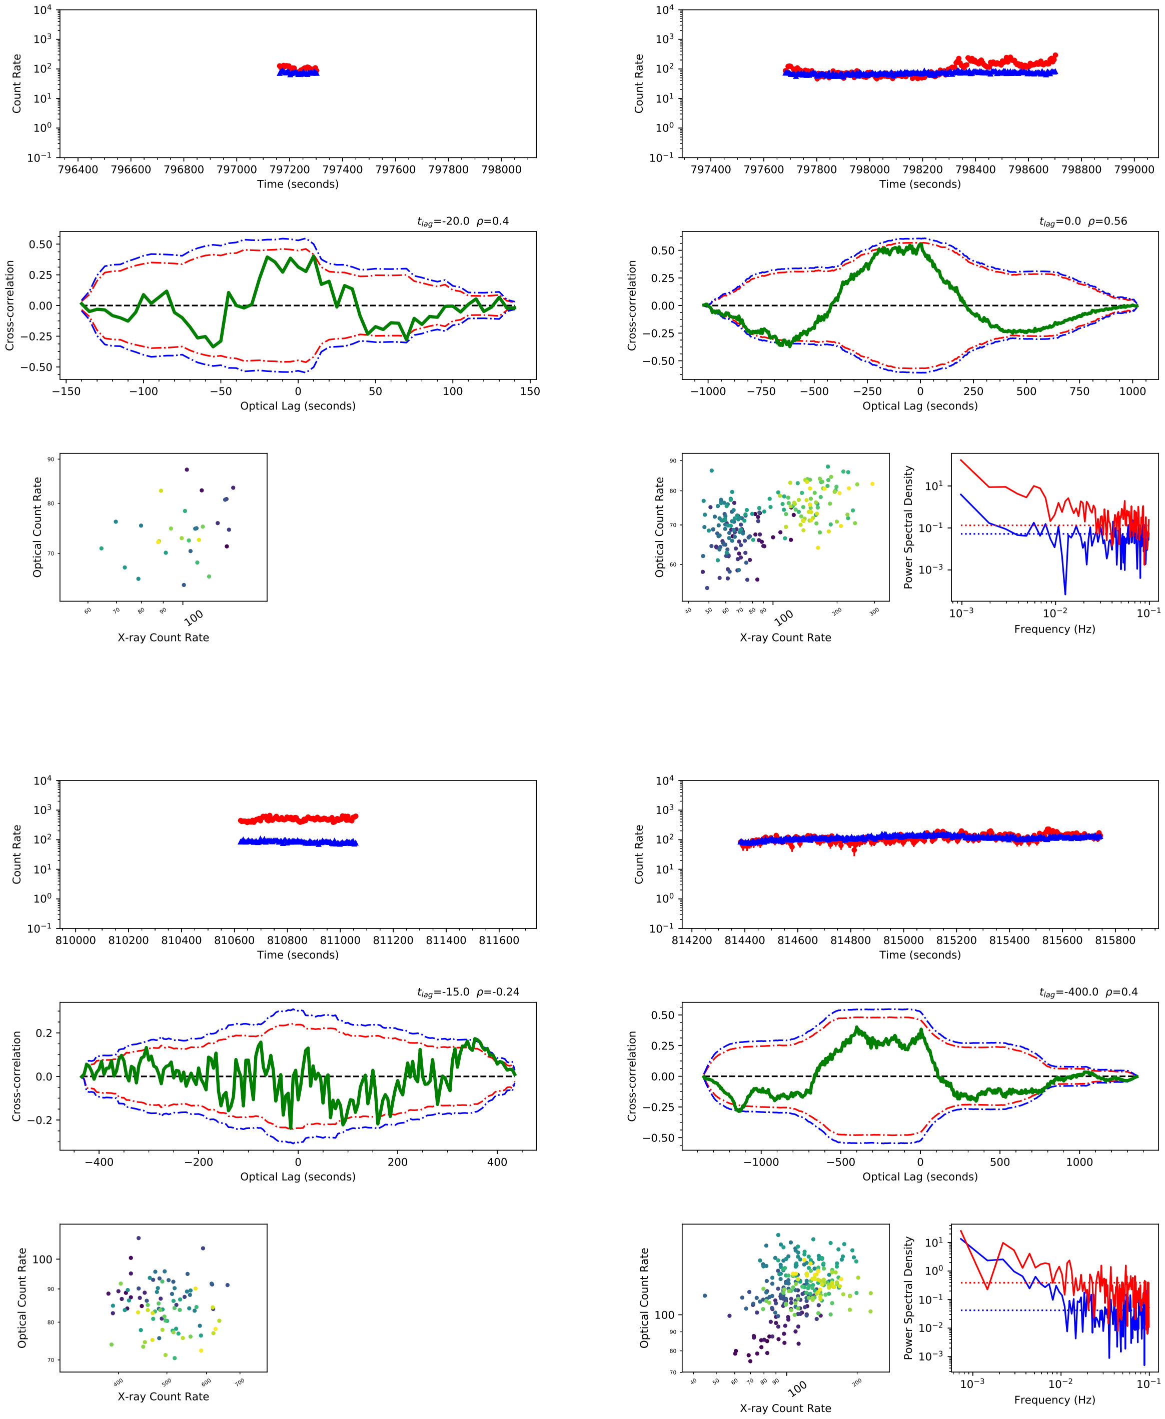


**Figure S.2 (Cont.).**

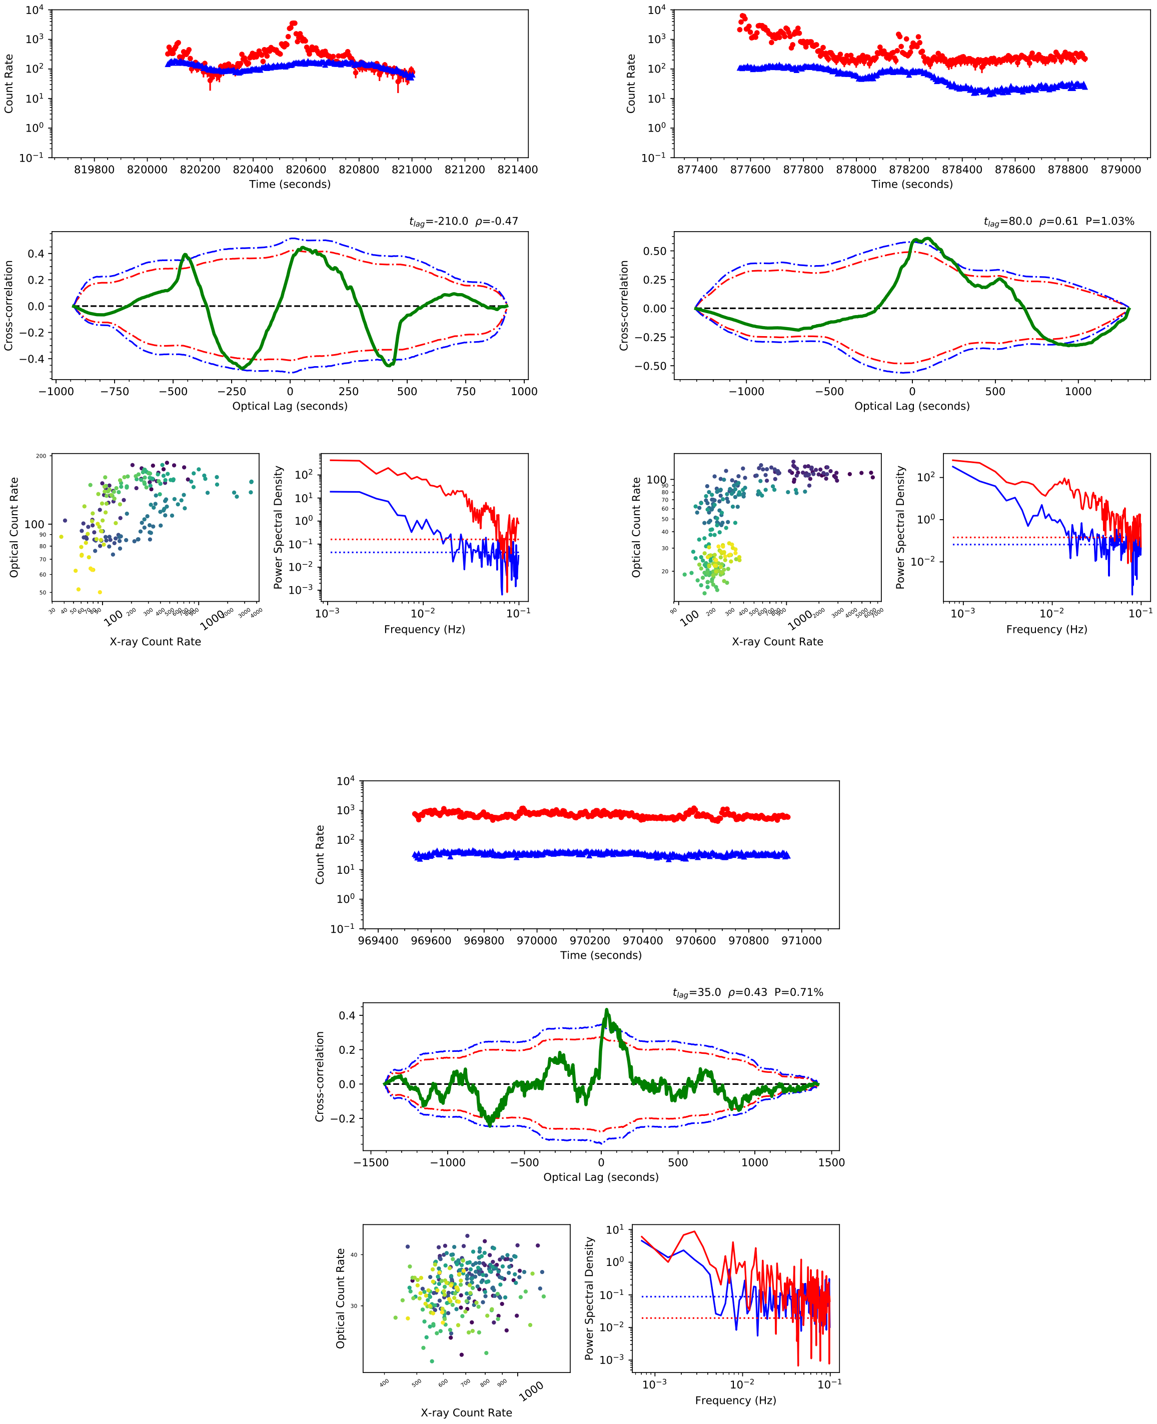


**Figure S.2 (Cont.).**
